# Supplementary material for: StyleFusion360: View-Consistent Head Stylization via Adaptive Style Modulation
Source: arXiv:2511.22411 source file (2026-06-24)
Supplement: Supplementary file 1 [file X_suppl.tex]

\clearpage
\setcounter{page}{1}
\maketitlesupplementary

%\section{Preliminaries}
%\noindent\textbf{Latent Diffusion Model.} 
%Diffusion models \cite{song2020ddim, ho2020ddpm, song2020score-based} are a class of generative models that produce target data samples by progressively denoising Gaussian noise $z_0$ over $T$ iterative time steps. Latent Diffusion Models (LDMs) \cite{rombach2022ldm} extend the diffusion framework by performing the denoising process in a compressed latent space \( E(I) \), where \( I \) denotes the input image. This is enabled by a pretrained autoencoder \( E(\cdot) \). The model is trained to reconstruct the latent representation by learning the denoising transition from \( z_T \sim \mathcal{N}(0, 1) \) to \( z_0 = E(I) \) with the following objective:

%\begin{equation}
%\mathcal{L}_{\text{LDM}} = 
%\mathbb{E}_{E(I), \epsilon, t} 
%\left[
%\left\| 
%\epsilon - \epsilon_\theta(z_t, t)
%\right\|_2^2
%\right],
%\end{equation}
%where \( z_t \) denotes the noisy latent representation at timestep \( t \), and \( \epsilon_\theta \) represents a trainable U-Net architecture composed of convolutional layers and self-/cross-attention modules (TransBlock). The denoised latent representation is decoded back into the image domain through \( I = D(z_0) \). Instead of relying on textual inputs as in traditional Text-to-Image (T2I) diffusion models, our method utilizes pose, content, and style appearance conditions, denoted as \( I_{\text{cam}} \), \( I_{\text{content}} \), and \( I_{\text{style}} \) to guide the image synthesis process. Therefore, the text prompt is omitted and not included in our model formulations.

\section{Dataset Pair Examples}

\cref{fig:gan_dataset_pairs} presents an example triplet from the \textit{Joker} style domain, consisting of a content image generated by a base 3D-GAN generator~\cite{an2023panohead}, a cross-identity style exemplar, and the corresponding ground-truth stylized output produced by a domain-adapted 3D-GAN model~\cite{Bilecen2025IdentityPreserving3DHeadStylization}. 
Note that the style exemplar itself is also generated using the same domain-adapted model. 
Using a style image from a different identity encourages a clearer separation between identity and style, enabling more effective disentanglement of content and stylistic attributes during training. 
For our dataset, we generate 150 samples for each of the six style domains, yielding a total of 900 training pairs. A representative subset of these samples is shown in \cref{fig:dataset_styles}.

\newcommand{\gandataset}[1]{%
\begin{tabular}[t]{@{}c@{}c@{}}
    \includegraphics[width=0.20\linewidth]{supplementary/gan_dataset/#1/view_00.png} &
    \raisebox{20pt}[0pt][0pt]{%
        \begin{tabular}{@{}c@{}}
            \includegraphics[width=0.10\linewidth]{supplementary/gan_dataset/#1/view_03.png} \\[-3pt]
            \includegraphics[width=0.10\linewidth]{supplementary/gan_dataset/#1/view_29.png}
        \end{tabular}%
    }
\end{tabular}%
}

\begin{figure}[t!]
    \centering
    \footnotesize
    \setlength{\tabcolsep}{1pt}

    \scalebox{1.0}{
        \begin{tabular}{ccc}
            \textbf{Content Image} & \textbf{Style Image} & \textbf{Ground Truth} \\
            \hline
            \noalign{\vskip 3pt}

            \gandataset{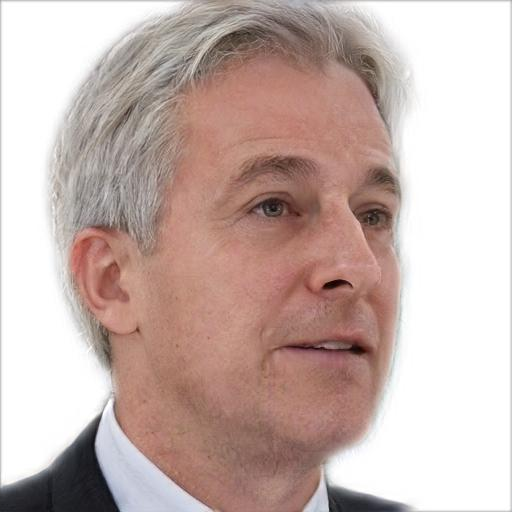} &
            \gandataset{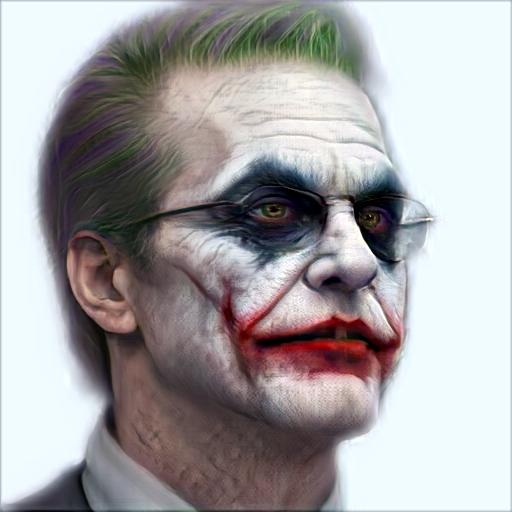} &
            \gandataset{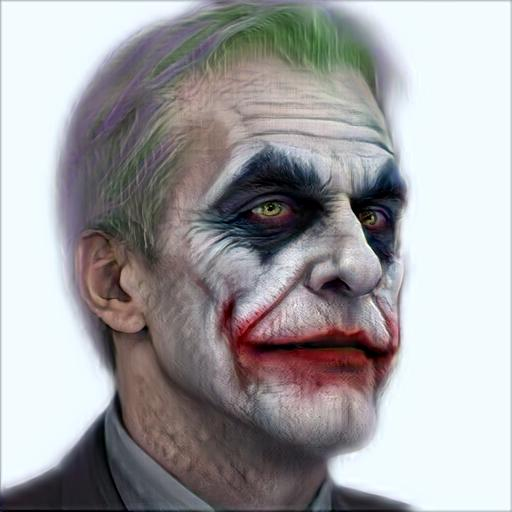}
        \end{tabular}
    }
    
    \caption{Dataset pairs used in our training.}
    \label{fig:gan_dataset_pairs}
    \vspace{-0.3cm}
\end{figure}

\begin{figure*}[t!]
    \centering
    \includegraphics[width=1.0\linewidth]{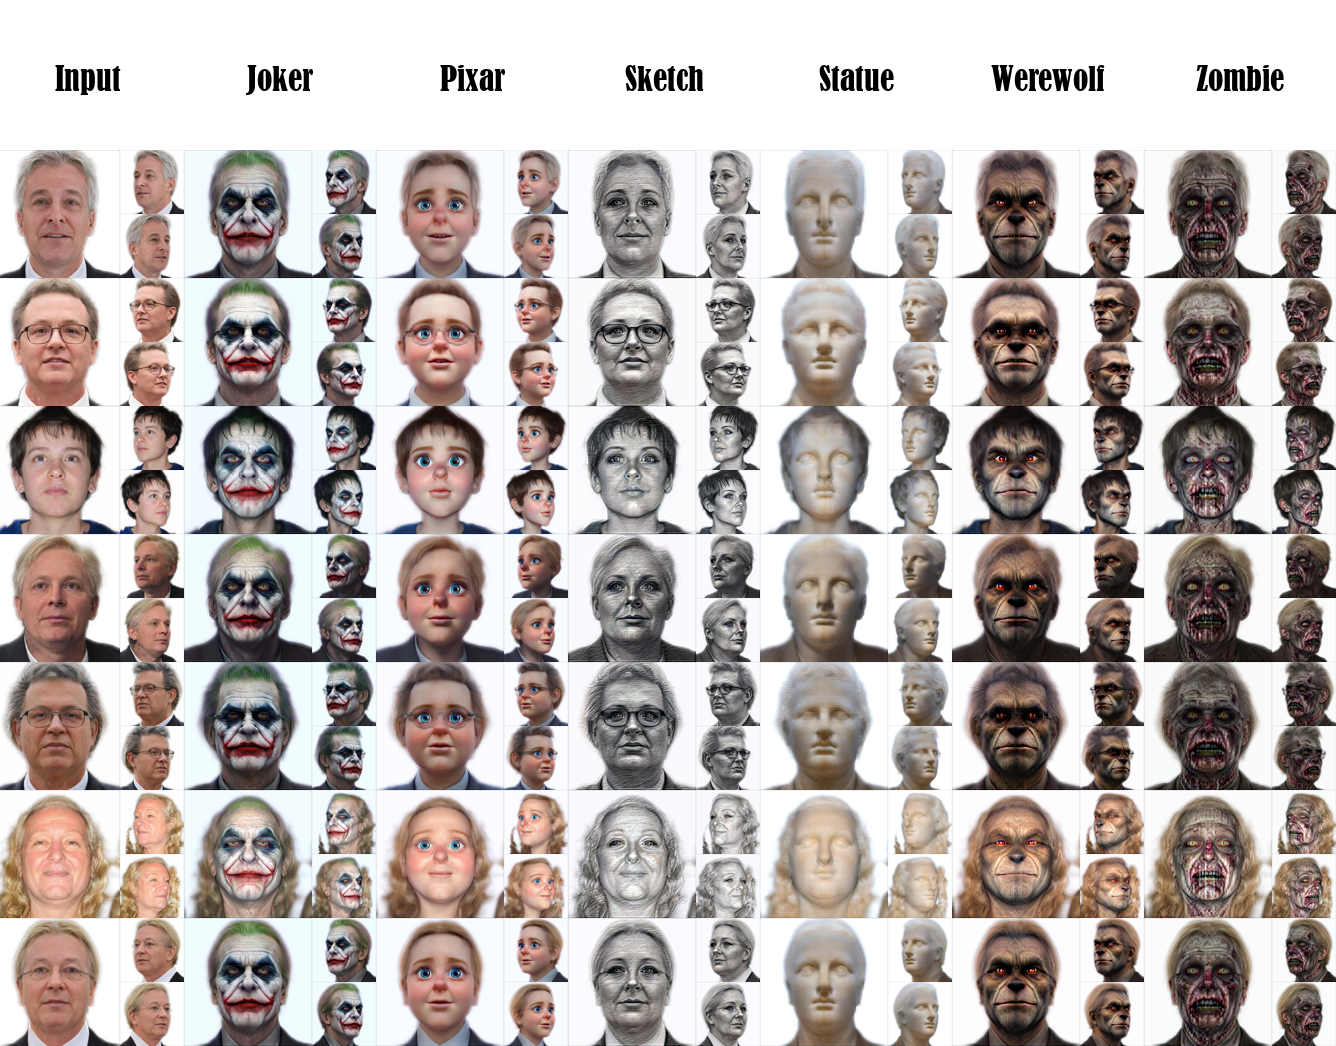}
      \vspace{-0.7cm}
    \caption{Dataset pair examples.}
    \label{fig:dataset_styles}
\end{figure*}

\section{Implementation Details}

\subsection{Training Setup}
We fine-tune the Style Appearance and View Consistency modules of our model on a synthetic 3D-GAN–generated stylized dataset for 800 iterations. The dataset includes six style categories: Joker, Pixar, Sketch, Statue, Werewolf, and Zombie. We use the AdamW optimizer with a learning rate of $10^{-5}$ and apply Classifier-Free Guidance (CFG) with a weight of 3.0. The batch size is 16, corresponding to the number of generated views per generation. All experiments are conducted on a single NVIDIA A100 GPU. We use $\tau = 1.05$ as the default key scaling value. 

\subsection{Baselines}

For diffusion-based stylization methods (IP2P and InstantID), we first stylize the input content image using a text-driven style prompt. The resulting stylized image is then passed through DiffPortrait360~\cite{gu2025diffportrait360} to synthesize multi-view stylized outputs.

We train the latent mapper of StyleCLIP \cite{patashnik2021styleclip} using the PanoHead generator. For StyleGAN-NADA \cite{gal2022stylegannada} and StyleGANFusion \cite{song2024DiffusionGuidedDomainAdaptation}, we rely on the official implementation of StyleGANFusion and adapt the generator backbone to PanoHead. In the case of StyleGANFusion, we use their EG3D configuration for PanoHead, and for StyleGAN-NADA \cite{gal2022stylegannada} we incorporate adaptive layer selection as described in the original method. DiffusionGAN3D \cite{lei2024diffusiongan3d} is implemented directly from the paper, as no official code is available. We preserve each baseline’s original hyperparameters, such as denoiser settings, noise schedule, learning rate, and optimizer, unless training instability requires adjustments.

\subsection{Quantitative Scores}
To evaluate our approach, we generate three reference image distributions using the Stable Diffusion pipeline. 
The first distribution is created by adding noise at timestep $t=25$ to the input images and denoising them for 50 steps with the corresponding style prompt using each baseline’s diffusion checkpoints. 
The resulting edited images serve as ground-truth targets for computing FID and CLIP similarity. 
The second distribution consists of the stylized outputs produced by the 3D head stylization methods, which we compare against the first distribution for FID and against matched pairs for CLIP scores. 
The third distribution contains the original, unedited images and is used to evaluate identity preservation (ID) and $\Delta D$. 
For ID preservation, we compute ArcFace-based~\cite{deng2019arcface} identity similarity between the stylized outputs and their corresponding input images. 
For depth consistency, $\Delta D$ is measured using depth maps estimated by the DepthAnything model~\cite{yang2024depthanything}. 
These metrics are computed by comparing images from the second and third distributions. 
\cref{fig:quantitative_eval_example} shows representative examples from all three distributions.

\begin{figure}[t!]
    \centering
    \footnotesize
    \setlength{\tabcolsep}{1pt}

    \scalebox{1.0}{
        \begin{tabular}{ccc}
            \textbf{Ours} & \textbf{Input} & \textbf{Ground Truth} \\
            \hline
            \noalign{\vskip 3pt}
            \includegraphics[width=0.30\linewidth]{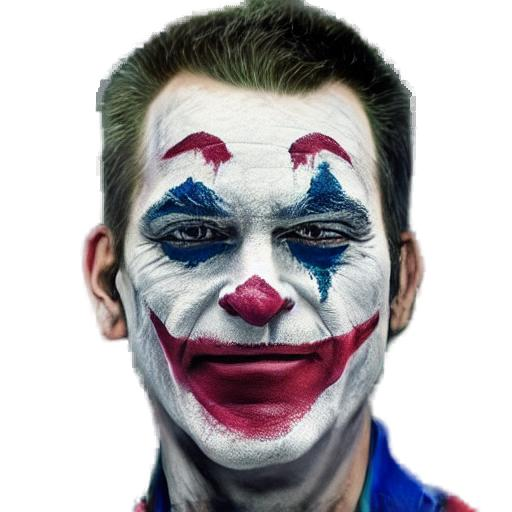} &
            \includegraphics[width=0.30\linewidth]{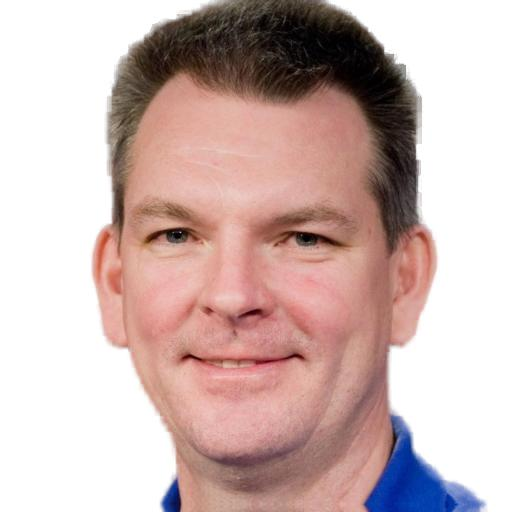} &
            \includegraphics[width=0.30\linewidth]{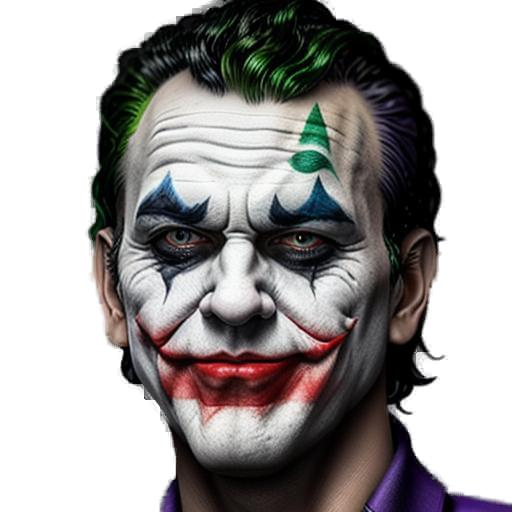} \\

            \includegraphics[width=0.30\linewidth]{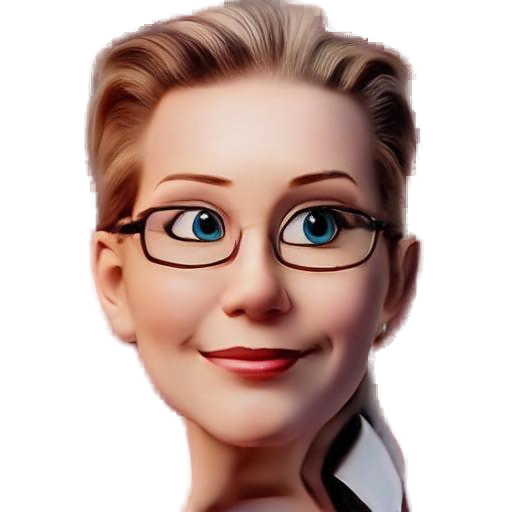} &
            \includegraphics[width=0.30\linewidth]{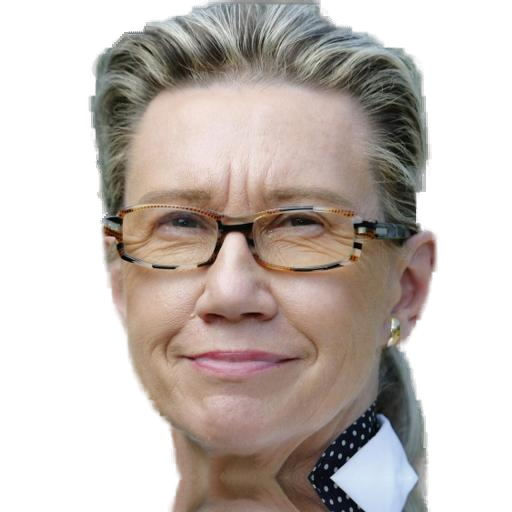} &
            \includegraphics[width=0.30\linewidth]{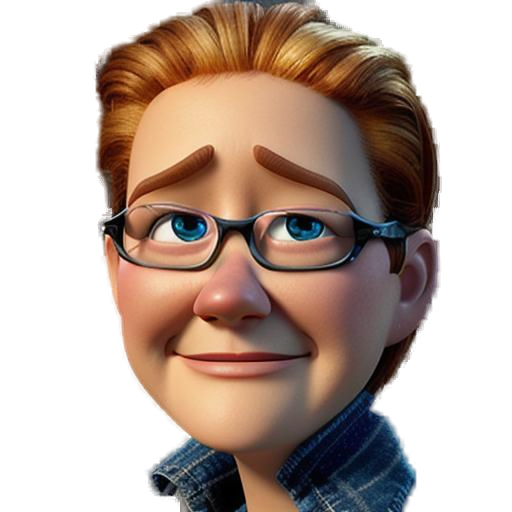} \\

        \end{tabular}
    }
    
    \caption{From left to right: a stylized image from the second distribution (outputs of our model), the corresponding unedited input image from the third distribution (used for evaluating identity preservation), and the edited result from the first distribution obtained by using the Stable Diffusion pipeline (used as the ground truth for FID and CLIP evaluations).
    \label{fig:quantitative_eval_example}
}
    \vspace{-0.3cm}
\end{figure}

\section{User Study}
We conducted a user study with \textbf{15 participants}, each of whom completed 
\textbf{18 comparison questions}. Options were randomly permuted to ensure fairness. In each question, the participant was shown:
\begin{itemize}
    \item the original content image,
    \item a style exemplar image
    \item stylized outputs produced by different methods.
\end{itemize}

Participants were asked to select the image that provides the \textbf{best balance of 
identity preservation and stylization}, i.e., the image that both retains recognizable 
identity and reflects the target style. We did not ask separate 
questions for identity and stylization; participants provided a single holistic judgment for each comparison.

The stylization results are provided in gif format. 
\begin{table}[t]
\centering
\resizebox{0.80\linewidth}{!}{
\begin{tabular}{l c}
\toprule
\textbf{Method} & \textbf{User Study (\%)} \\
\midrule
IP2P~\cite{brooks2023ip2p} & 6.7\% \\
StyleGAN-Fusion~\cite{song2024DiffusionGuidedDomainAdaptation} & 2.4\% \\
Bilecen \etal~\cite{Bilecen2025IdentityPreserving3DHeadStylization} & 12.7\% \\
\textbf{Ours} & \textbf{78.2\%} \\
\bottomrule
\end{tabular}}
\caption{User study preference on the FFHQ dataset, aggregated over 270 responses 
(15 participants $\times$ 18 questions). Higher values indicate stronger user preference.}
\label{tab:userstudy}
\end{table}

As shown in Table~\ref{tab:userstudy}, participants preferred our method in 
\textbf{78.2\%} of all comparisons, indicating that our approach achieves the most favorable perceptual trade-off between identity retention and stylistic fidelity.

\section{Stylization-Identity Trade-Off Analysis}

As shown in \cref{tab:clip_id_separated} and \cref{fig:stylization_view_comparison}, the quantitative trends reveal a clear stylization--identity trade-off among baseline methods. InstantID~\cite{wang2024instantid} consistently reports high identity similarity scores across all styles; however, these metrics reflect its generally weak stylization capability rather than true identity preservation under meaningful edits. Because InstantID applies only subtle tonal changes, the output remains close to the input image, inflating ID scores while failing to capture the intended style.

IP2P~\cite{brooks2023ip2p} shows more inconsistent behavior across domains. For styles such as \emph{Sketch}, \emph{Statue}, and \emph{Werewolf}, IP2P performs filter-like transformations that preserve most facial structure, leading to high identity scores in \cref{tab:clip_id_separated}. In contrast, for semantically demanding styles such as \emph{Joker} and \emph{Pixar}, IP2P introduces stronger but less controlled changes that reduce identity similarity while still failing to deliver faithful stylization.

These quantitative observations are clearly reflected in the qualitative comparisons in Fig.~\ref{fig:stylization_view_comparison}. When integrated into the DiffPortrait360 pipeline for novel-view synthesis, both IP2P and InstantID struggle to maintain consistency across viewpoints. Their limited or unstable stylization does not generalize well to unseen views, frequently resulting in degraded back-view quality, texture collapse, and Janus-like artifacts where facial features incorrectly appear on the back of the head. These multi-view failures further indicate that high ID scores in \cref{tab:clip_id_separated} do not correspond to robust stylization, but rather to insufficient or inconsistent transformations.

In contrast, our approach delivers semantically aligned, domain-consistent stylizations that remain coherent across all viewpoints. As evidenced by both \cref{tab:clip_id_separated} and Fig.~\ref{fig:stylization_view_comparison}, our method achieves a more favorable balance, producing strong stylization while maintaining significantly better identity retention and multiview consistency than prior methods.

\begin{figure}[t]
    \centering
    \begin{subfigure}{\linewidth}
        \centering
        \includegraphics[width=\linewidth]{supplementary/plots/id_vs_key_scaling.pdf}
        \caption{Identity score vs.\ Key Scaling.}
        \label{fig:key_scaling_id}
    \end{subfigure}
    \hfill
    \begin{subfigure}{\linewidth}
        \centering
        \includegraphics[width=\linewidth]{supplementary/plots/clip_vs_key_scaling.pdf}
        \caption{CLIP score vs.\ Key Scaling}
        \label{fig:key_scaling_clip}
    \end{subfigure}

    \caption{
    Analysis of the effect of Key Scaling on stylization and identity preservation for Statue style on the RenderMe360 dataset.  
    Increasing the scaling factor $\tau$ enhances stylistic alignment (higher CLIP) but leads to reduced identity similarity (lower ID), demonstrating a clear stylization--identity trade-off.
    }
    \label{fig:key_scaling_ablation}
\end{figure}

\begin{figure}[t]
    \centering
    \footnotesize
    \setlength{\tabcolsep}{1pt}

    \scalebox{1.0}{
        \begin{tabular}{ccc}
            \textbf{Frontal View} & \textbf{View-1} & \textbf{View-2} \\
            \hline
            \noalign{\vskip 3pt}
            \includegraphics[width=0.30\linewidth]{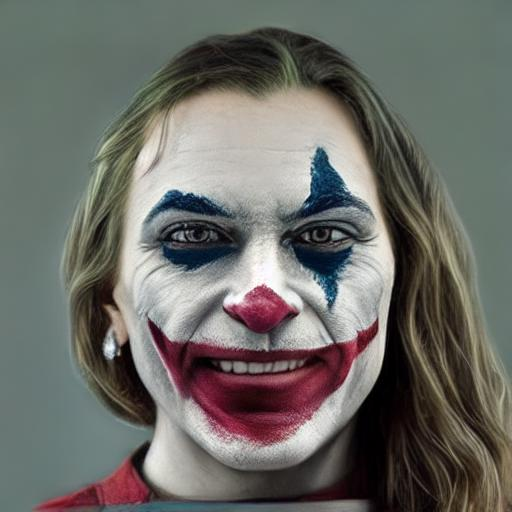} &
            \includegraphics[width=0.30\linewidth]{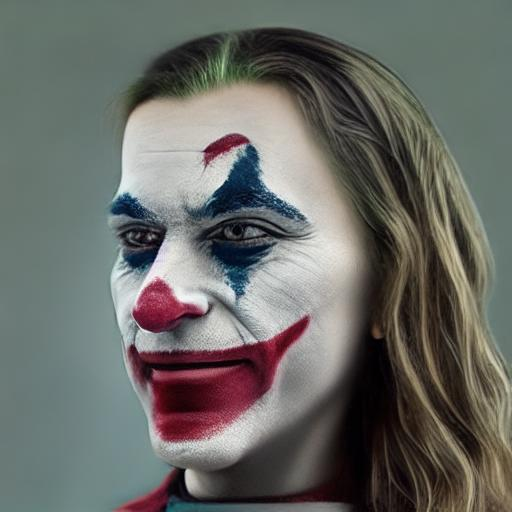} &
            \includegraphics[width=0.30\linewidth]{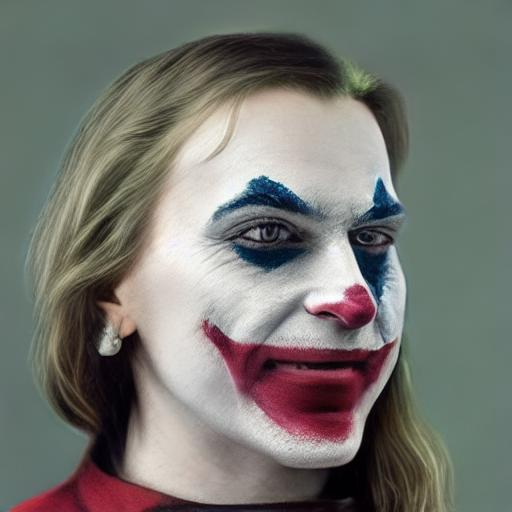} \\

            \includegraphics[width=0.30\linewidth]{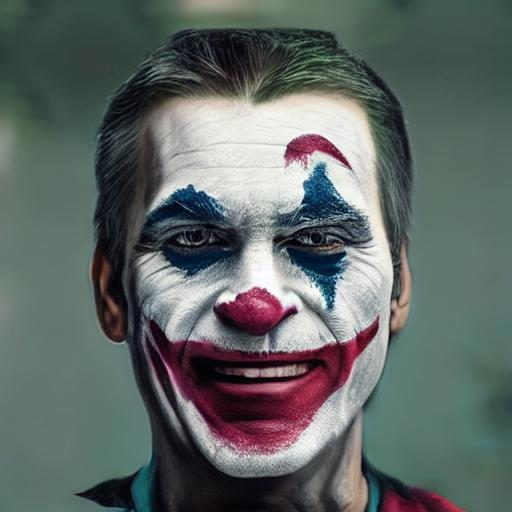} &
            \includegraphics[width=0.30\linewidth]{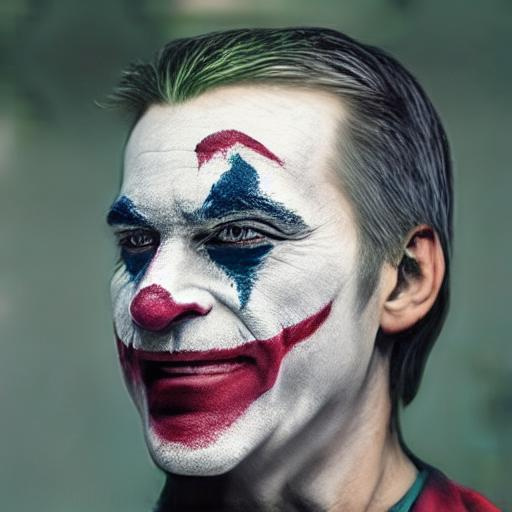} &
            \includegraphics[width=0.30\linewidth]{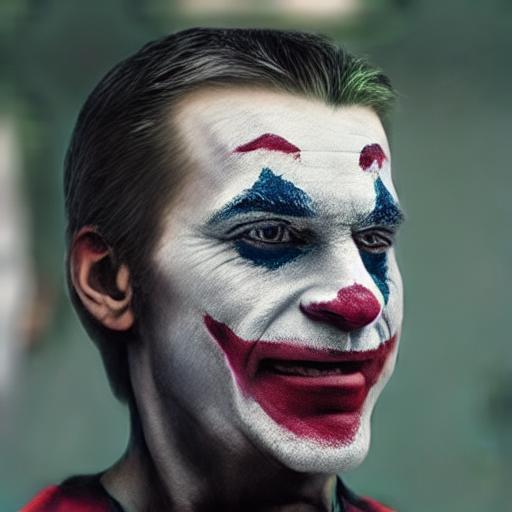} \\

        \end{tabular}
    }
    
    \caption{
Limitations of our method. In rare cases, certain style elements may not remain fully consistent across views. 
As shown, the Joker eyebrow appearance exhibits slight inconsistency between angles. 
}
\label{fig:joker_limitation}
    \vspace{-0.3cm}
\end{figure}

\begin{table*}[t]
\centering
\resizebox{\textwidth}{!}{
\begin{tabular}{lcc|cc|cc|cc|cc}
\toprule
& \multicolumn{2}{c|}{\textbf{Joker}} 
& \multicolumn{2}{c|}{\textbf{Pixar}} 
& \multicolumn{2}{c|}{\textbf{Sketch}} 
& \multicolumn{2}{c|}{\textbf{Statue}} 
& \multicolumn{2}{c}{\textbf{Werewolf}} \\
\cmidrule(lr){2-3}
\cmidrule(lr){4-5}
\cmidrule(lr){6-7}
\cmidrule(lr){8-9}
\cmidrule(lr){10-11}
\textbf{Method} 
& CLIP $\uparrow$ & ID $\uparrow$
& CLIP $\uparrow$ & ID $\uparrow$
& CLIP $\uparrow$ & ID $\uparrow$
& CLIP $\uparrow$ & ID $\uparrow$
& CLIP $\uparrow$ & ID $\uparrow$ \\
\midrule
IP2P~\cite{brooks2023ip2p}
& 0.8832 & 0.2237 
& 0.8096 & 0.2046
& 0.6592 & 0.7334
& 0.7693 & 0.5829
& 0.7782 & 0.4554 \\
InstantID~\cite{wang2024instantid}
& 0.6997 & 0.4662
& 0.6621 & 0.4857
& 0.6994 & 0.4946
& 0.7627 & 0.4706
& 0.6589 & 0.4915 \\
StyleCLIP~\cite{patashnik2021styleclip}
& 0.7821 & 0.1239
& 0.7481 & 0.1753
& 0.7413 & 0.1845
& 0.7123 & 0.2059
& 0.6634 & 0.1170 \\
StyleGAN-Fusion~\cite{song2024DiffusionGuidedDomainAdaptation}
& 0.8452 & 0.1105
& 0.7813 & 0.2211
& 0.7652 & 0.1636
& 0.8232 & 0.1385
& 0.8008 & 0.1477 \\
StyleGANNADA~\cite{gal2022stylegannada}
& 0.8035 & 0.1728
& 0.7710 & 0.1873
& 0.7375 & 0.1666
& 0.7302 & 0.0934
& 0.7611 & 0.1329 \\
DiffusionGAN3D~\cite{lei2024diffusiongan3d}
& 0.7884 & 0.2298
& 0.8077 & 0.1545
& 0.6745 & 0.1707
& 0.8450 & 0.1552
& 0.7856 & 0.2036 \\
Bilecen \etal~\cite{Bilecen2025IdentityPreserving3DHeadStylization}
& 0.8617 & 0.1877
& 0.8211 & 0.2336
& 0.7577 & 0.2752
& 0.8197 & 0.1952
& 0.8444 & 0.1755 \\
\textbf{Ours}
& 0.8334 & 0.3132
& 0.7868 & 0.3500
& 0.7578 & 0.3428
& 0.8090 & 0.3529
& 0.7865 & 0.3186 \\
\textbf{Ours + Key Scaling}
& 0.8649 & 0.1843
& 0.8116 & 0.2598
& 0.7466 & 0.1945
& 0.8182 & 0.2031
& 0.8545 & 0.1611 \\
\bottomrule
\end{tabular}}
\caption{CLIP and identity similarity scores across \textbf{Joker}, \textbf{Pixar}, \textbf{Sketch}, \textbf{Statue}, and \textbf{Werewolf} style domains on the FFHQ dataset.}
\label{tab:clip_id_separated}
\end{table*}

% =====================================================
\newcommand{\vcenterimg}[2]{%
    \begin{tabular}[c]{@{}c@{}}\includegraphics[width=#1]{#2}\end{tabular}%
}

% =====================================================
% 2. Updated \localedit Macro
% =====================================================
\newcommand{\localedit}[2]{%
\begin{tabular}[c]{@{}c@{}c@{}}
    \vcenterimg{0.16\linewidth}{figures/local_edit/#1/#2/00.jpg} &
    \begin{tabular}[c]{@{}c@{}}
        \vcenterimg{0.08\linewidth}{figures/local_edit/#1/#2/03.jpg} \\[-2pt]
        \vcenterimg{0.08\linewidth}{figures/local_edit/#1/#2/29.jpg}
    \end{tabular}%
\end{tabular}%
}

\begin{figure}[t!]
    \centering
    \footnotesize
    \setlength{\tabcolsep}{0.5pt}

    % =====================================================
    % (a) Upper Subfigure — Local Stylization Results
    % =====================================================
    \begin{subfigure}{\linewidth}
        \centering
        \begin{tabular}{ccccc}
            Style Image & Input & Output & Input & Output \\
            \hline
            \noalign{\vskip 5pt}

            % All standalone images are now wrapped in \vcenterimg
            \vcenterimg{0.16\linewidth}{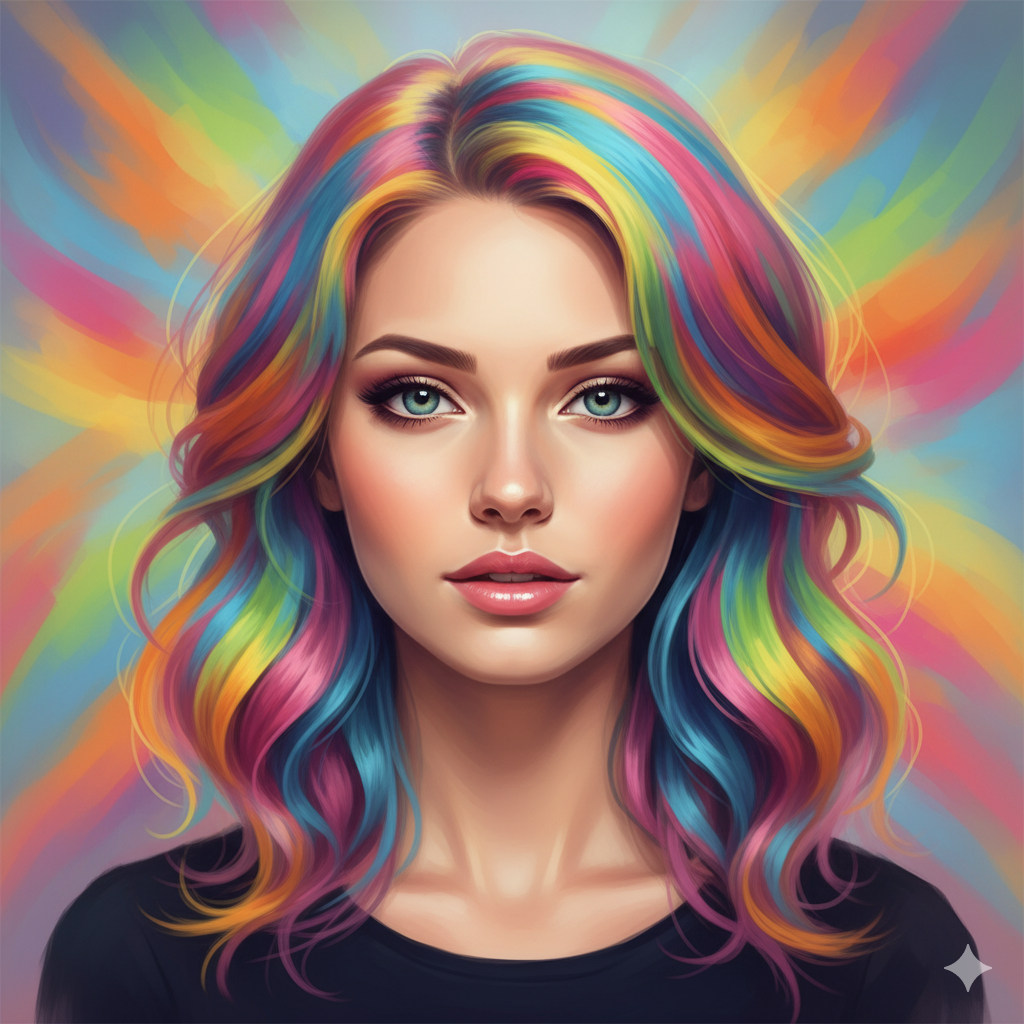} &
            \vcenterimg{0.16\linewidth}{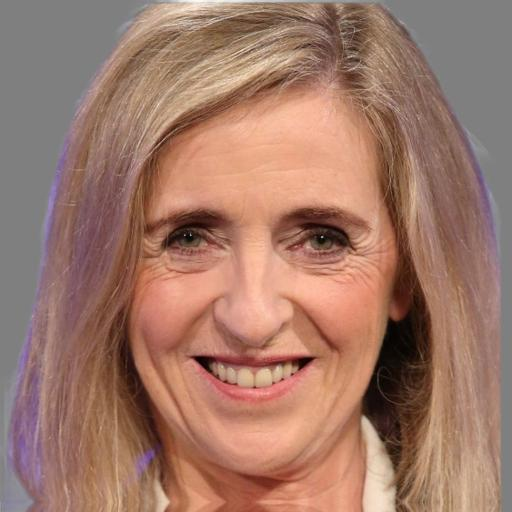} &
            \localedit{colorful_hair}{00251} &
            \vcenterimg{0.16\linewidth}{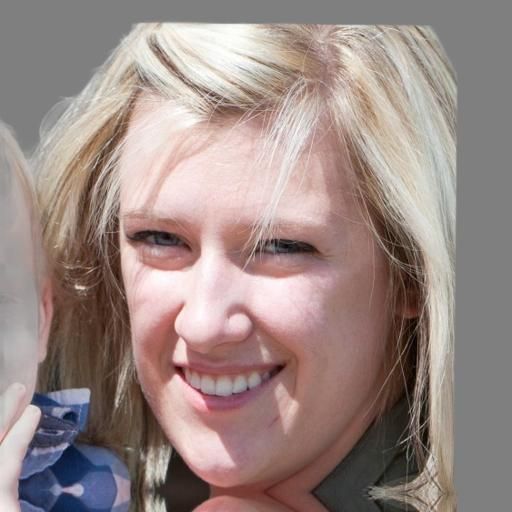} &
            \localedit{colorful_hair}{00138} \\ \noalign{\vskip 4pt}

            \vcenterimg{0.16\linewidth}{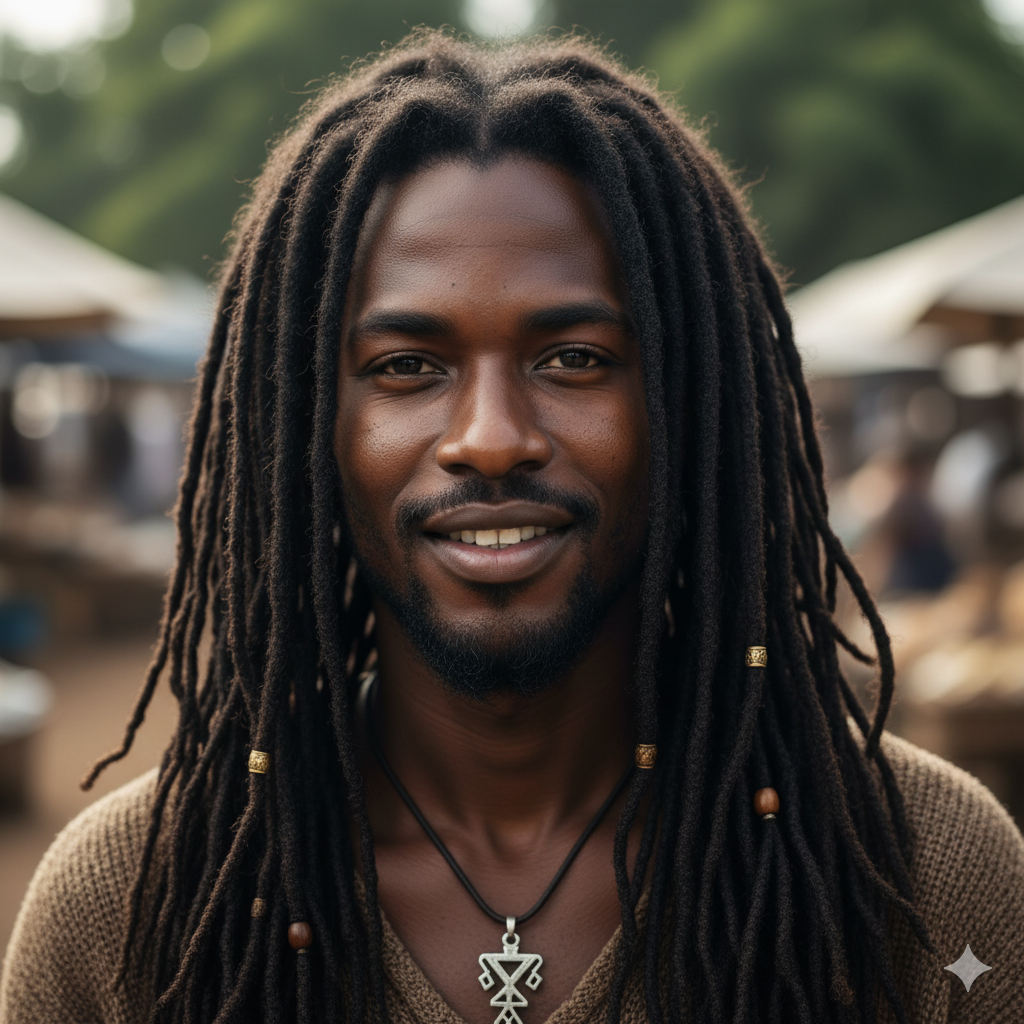} &
            \vcenterimg{0.16\linewidth}{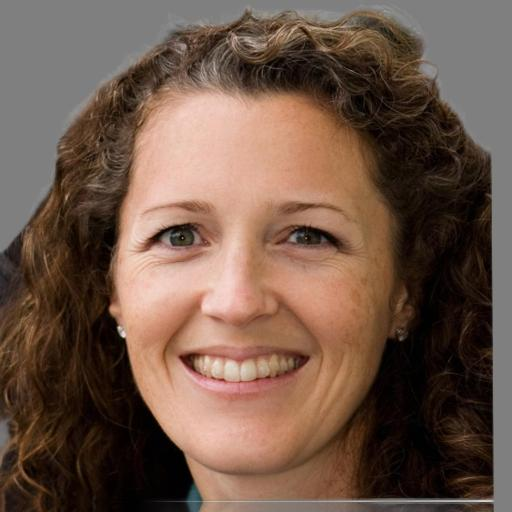} &
            \localedit{dreadlocks}{00207} &
            \vcenterimg{0.16\linewidth}{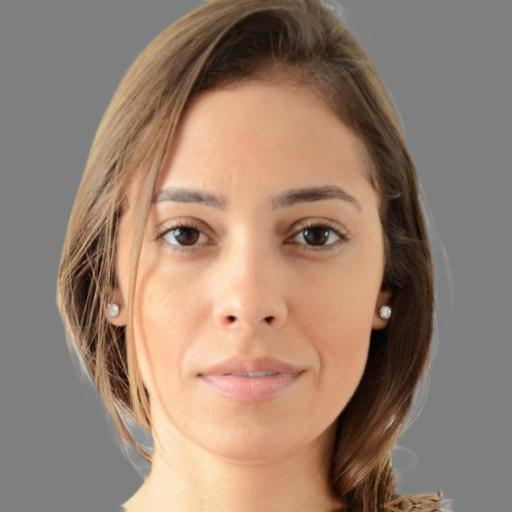} &
            \localedit{dreadlocks}{00200} \\ \noalign{\vskip 4pt}

            \vcenterimg{0.16\linewidth}{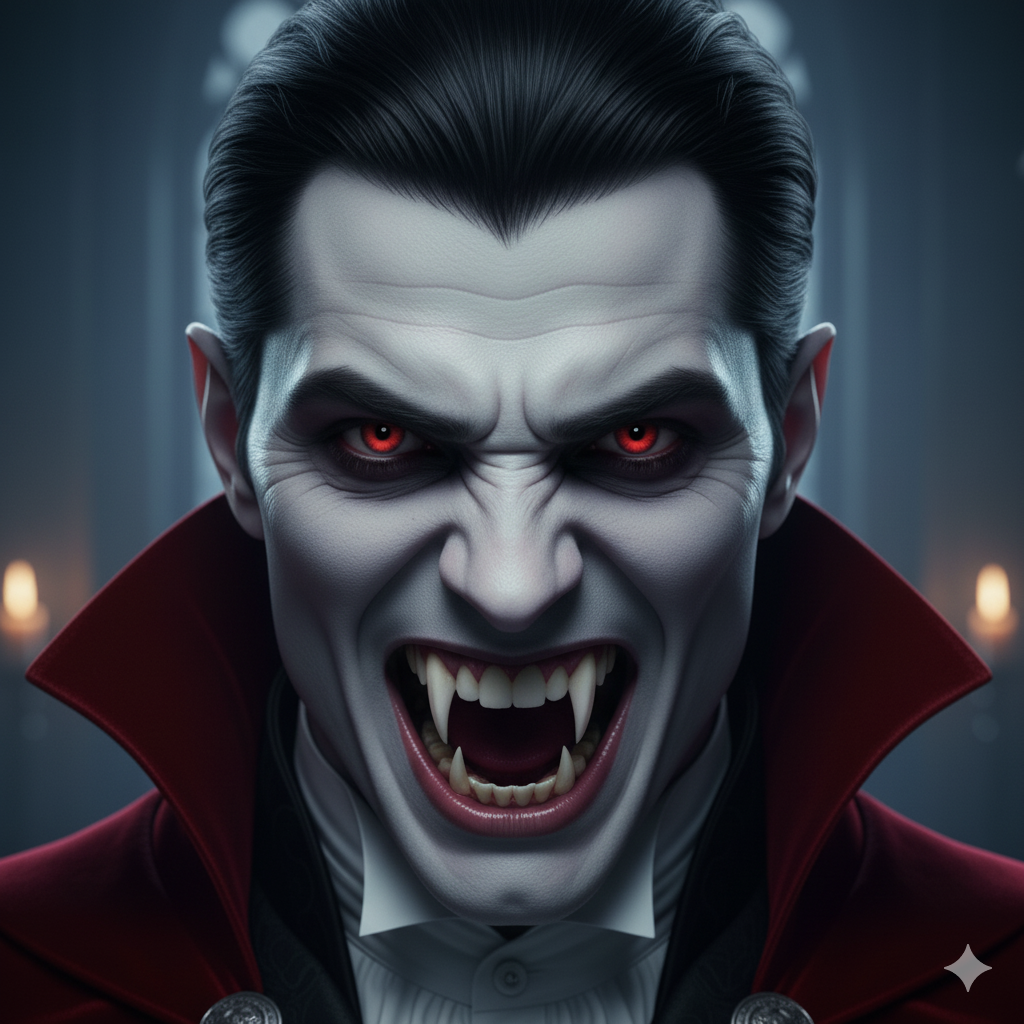} &
            \vcenterimg{0.16\linewidth}{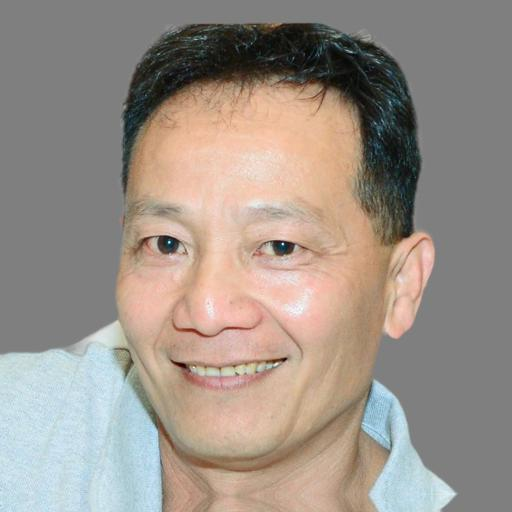} &
            \localedit{vampire}{00176} &
            \vcenterimg{0.16\linewidth}{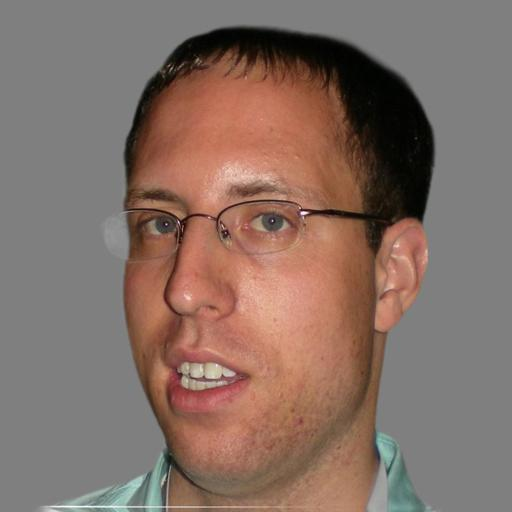} &
            \localedit{vampire}{00235} \\ \noalign{\vskip 4pt}

            \vcenterimg{0.16\linewidth}{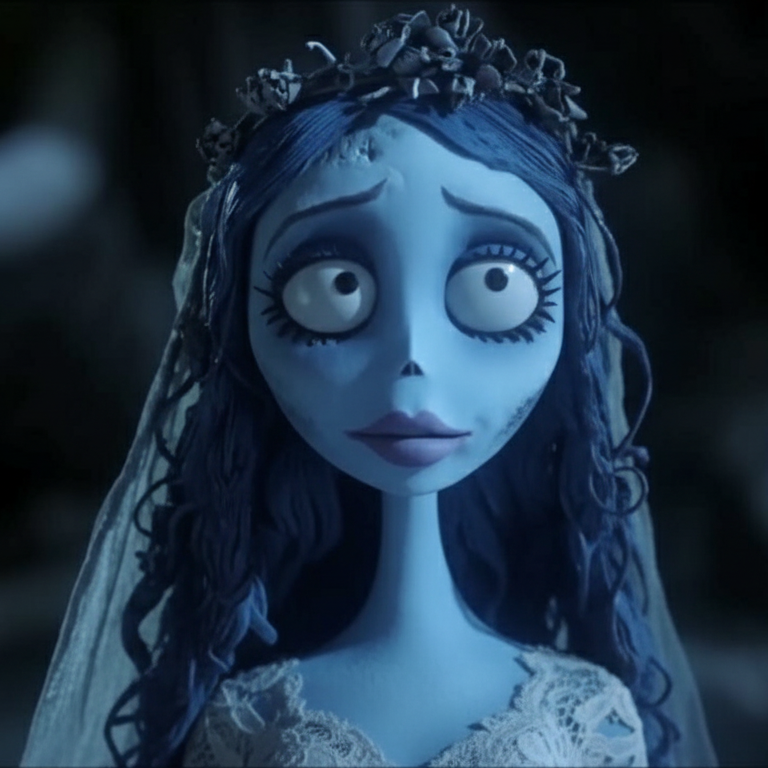} &
            \vcenterimg{0.16\linewidth}{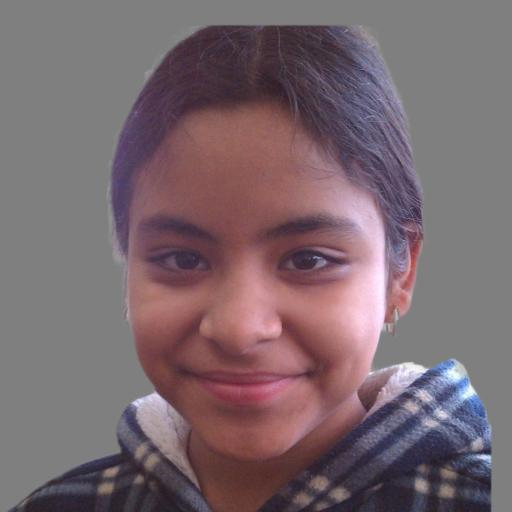} &
            \localedit{corpse_bride}{00116} &
            \vcenterimg{0.16\linewidth}{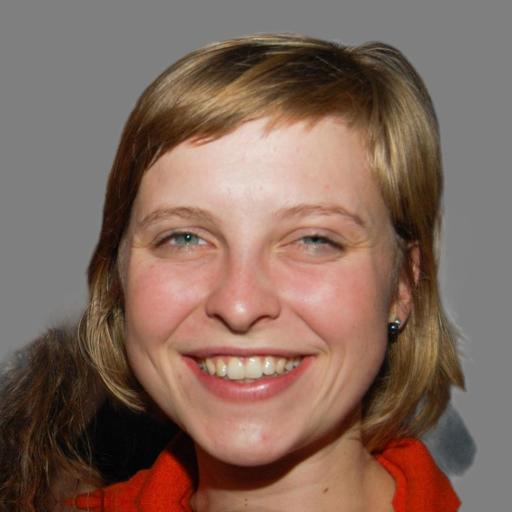} &
            \localedit{corpse_bride}{00167} \\
        \end{tabular}
        \caption{Local stylization results across different styles.}
    \end{subfigure}

    \vspace{0.4cm}

    % =====================================================
    % (b) Lower Subfigure — Multi-style Example
    % =====================================================
    \begin{subfigure}{\linewidth}
        \centering
        \begin{tabular}{cccc}
            Input & Style 1 & Style 2 & Output \\
            \noalign{\vskip 3pt}
            \vcenterimg{0.20\linewidth}{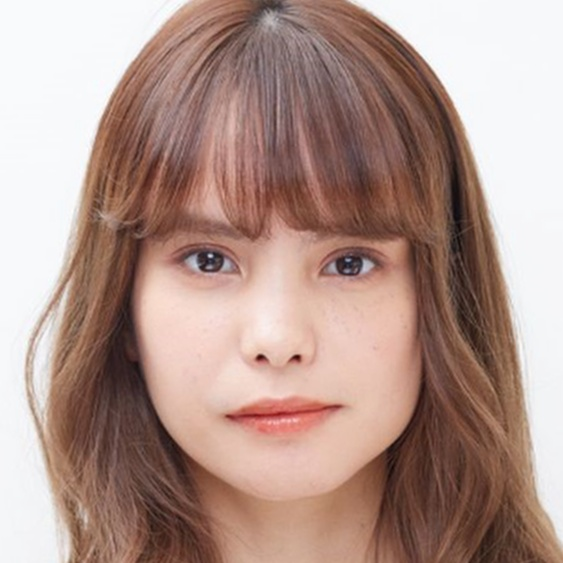} &
            \vcenterimg{0.20\linewidth}{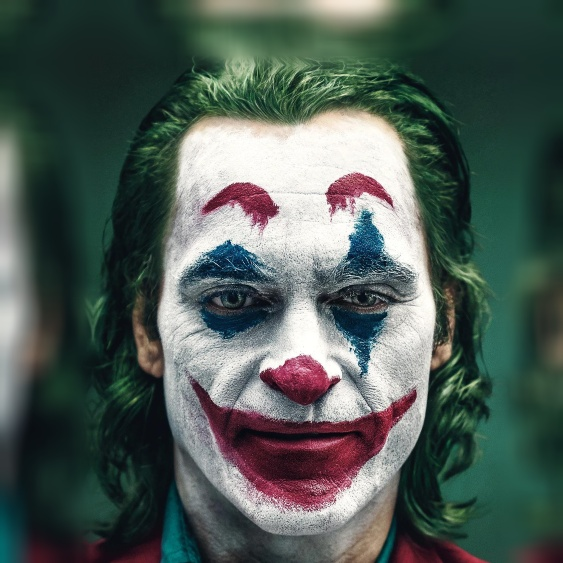} &
            \vcenterimg{0.20\linewidth}{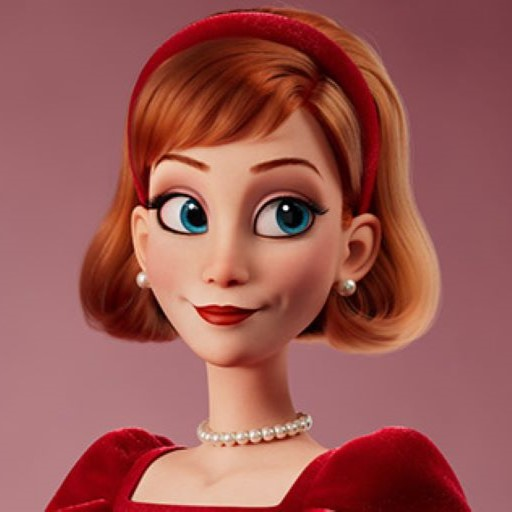} &
            \begin{tabular}[c]{@{}c@{}c@{}}
                \vcenterimg{0.20\linewidth}{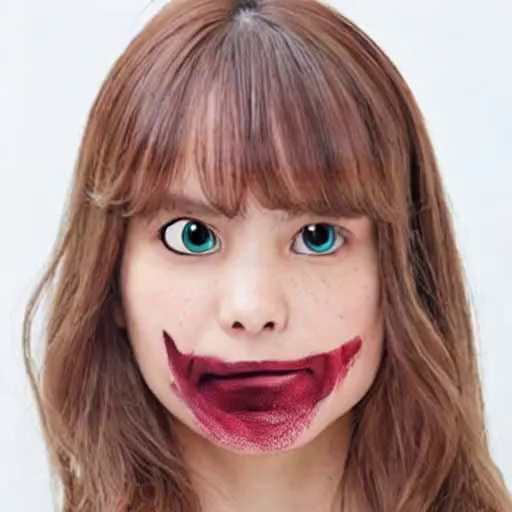} &
                \begin{tabular}[c]{@{}c@{}}
                    \vcenterimg{0.1\linewidth}{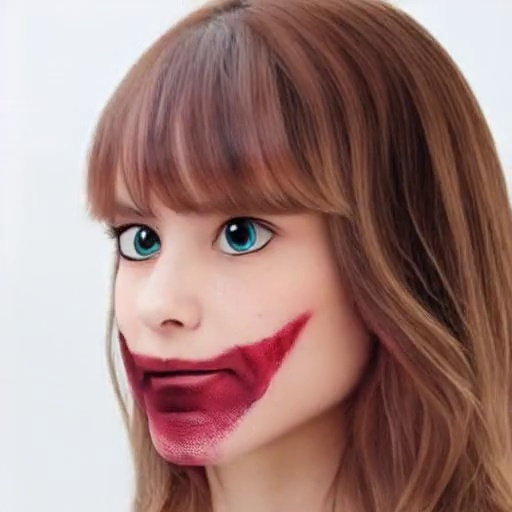} \\[-3pt]
                    \vcenterimg{0.1\linewidth}{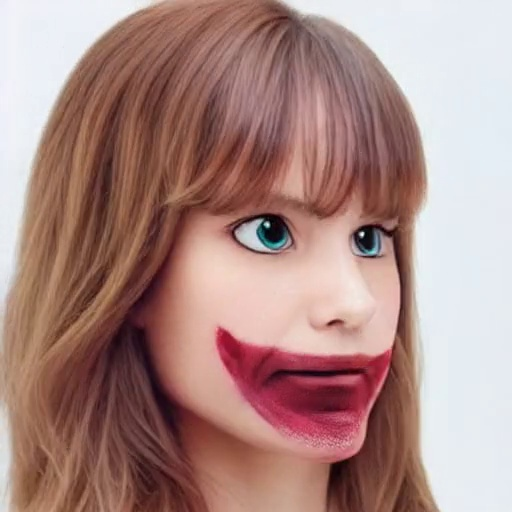}
                \end{tabular}%
            \end{tabular} \\
        \end{tabular}
        \caption{Example of combining two different style references.}
    \end{subfigure}
    \caption{(a) Local stylization results. (b) Multi-style local editing.}
    \label{fig:local_style_combined}
    
\end{figure}

\begin{figure*}[t!]
    \centering
    \includegraphics[width=1.0\linewidth]{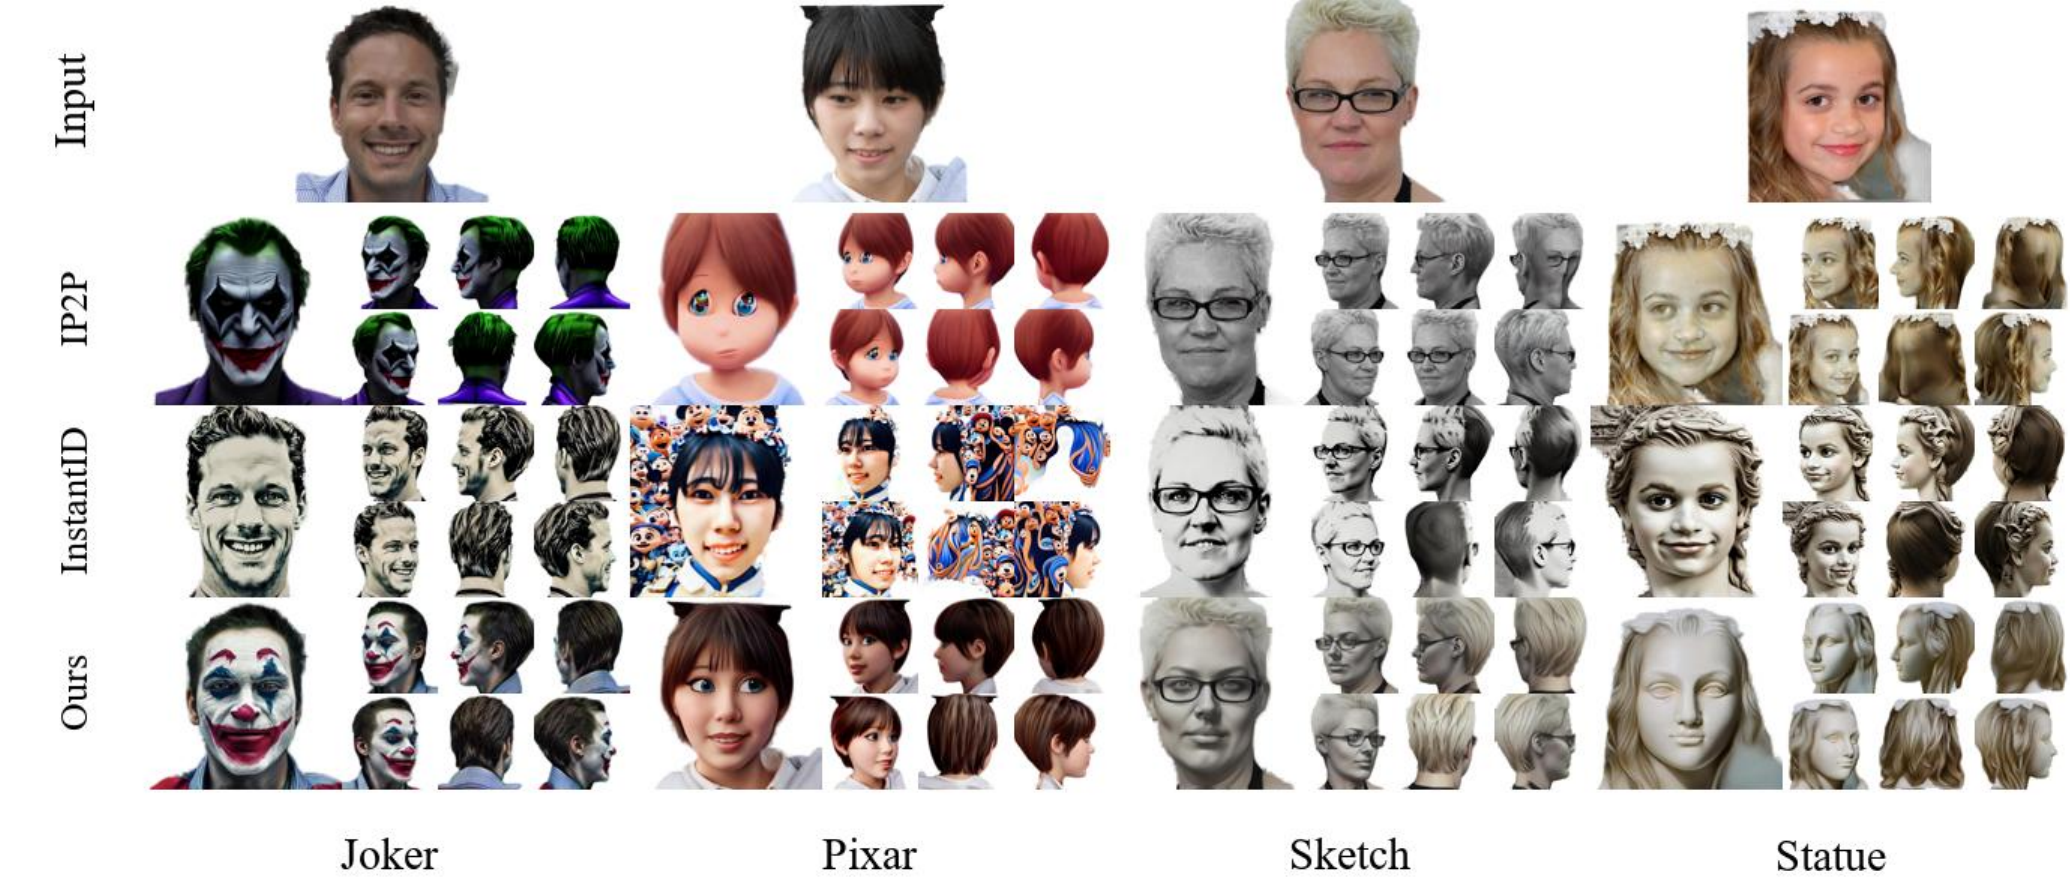}
      \vspace{-0.7cm}
    \caption{
    Qualitative illustration of the stylization–identity trade-off and view-consistency behavior across methods for Joker, Pixar, Sketch, and Statue domains. 
    IP2P applies filter-like adjustments for some domains such as Sketch and Statue (leading to inflated ID scores) but introduces uncontrolled changes for others (e.g., Joker and Pixar), causing identity drift. 
    When combined with DiffPortrait360 for novel-view synthesis, both methods frequently fail to maintain consistent 3D structure, showing back-view degradation and Janus-like artifacts. InstantID produces only subtle tonal modifications, resulting in weak stylization but high identity scores as reflected in \cref{tab:clip_id_separated}. 
    Our method achieves strong, semantically aligned stylization with stable identity across all viewpoints and robust multi-view geometry.
    }
    \label{fig:stylization_view_comparison}
\end{figure*}

\subsection{Effect of Key Scaling on Stylization and Identity Preservation}

To analyze the impact of the proposed Key Scaling mechanism, we evaluate identity similarity and CLIP-based style alignment across different scaling values. As shown in Fig.~\ref{fig:key_scaling_id}, increasing the scaling factor consistently lowers identity similarity: the ID score drops from $0.28$ at $\tau\!=\!1.0$ to $0.13$ at $\tau\!=\!1.07$, indicating stronger deviation from the input identity as stylistic cues are amplified in attention. Conversely, Fig.~\ref{fig:key_scaling_clip} shows that CLIP alignment improves with larger scaling values, peaking at $\tau\!=\!1.07$ before slightly declining at $\tau\!=\!1.10$. 

Overall, Key Scaling provides a controllable trade-off between stylization strength and identity preservation. Smaller values retain identity but weaken stylization, whereas larger values yield stronger style fidelity at the cost of identity drift. We select $\tau\!=\!1.05$ as a balanced setting that offers improved stylization with manageable identity loss.

%\begin{table}[t]
%\centering
%\resizebox{0.50\textwidth}{!}{
%\begin{tabular}{lcc|cc}
%\toprule
% & \multicolumn{2}{c|}%{\textbf{FFHQ}} 
% & \multicolumn{2}{c}{\textbf{RenderMe360}} \\
%\cmidrule(lr){2-3} \cmidrule(lr){4-5}
%\textbf{Method} 
%& CLIP $\uparrow$ 
%& ID $\uparrow$
%& CLIP $\uparrow$ 
%& ID $\uparrow$ \\
%\midrule
%IP2P~\cite{brooks2023ip2p}                     & 0.7799 & 0.4400 & 0.7446 & 0.5569 \\
%InstantID~\cite{wang2024instantid}            & 0.6966 & \textbf{0.4817} & 0.6549 & \textbf{0.6910} \\
%StyleCLIP~\cite{patashnik2021styleclip}       & 0.7294 & 0.1613 & 0.6816 & 0.1775 \\
%StyleGAN-Fusion~\cite{song2024DiffusionGuidedDomainAdaptation} 
%& 0.8031 & 0.1563 & 0.7526 & 0.1507 \\
%StyleGANNADA~\cite{gal2022stylegannada}       & 0.7607 & 0.1506 & 0.7051 & 0.1596 \\
%Diffusion3D~\cite{lei2024diffusiongan3d}      & 0.7802 & 0.1828 & 0.7329 & 0.2628 \\
%Bilecen \etal~\cite{Bilecen2025IdentityPreserving3DHeadStylization} 
% & 0.8209 & 0.2134 & 0.7762 & 0.2186 \\
%\textbf{Ours}                                  & 0.7967 & 0.3220 & 0.7709 & 0.3855 \\
%\textbf{Ours + Key Scaling}                    & \textbf{0.8237} & 0.1973 & \textbf{0.8000} & 0.2137 \\
%\bottomrule
%\end{tabular}}
%\caption{CLIP and identity similarity scores on \textbf{FFHQ} and \textbf{RenderMe360}}
%\label{tab:clip_id_separated}
%\end{table}

\section{Limitations}

Although our method achieves strong multi-view consistency in the vast majority of cases, certain challenging styles can still introduce localized inconsistencies across viewpoints. As illustrated in Fig.~\ref{fig:joker_limitation}, the stylized Joker eyebrows appear coherent in some views but exhibit slight deformation or misalignment when rendered from other angles. These artifacts typically arise when the target style contains highly exaggerated or fine-grained facial elements that place strong demands on cross-view geometric alignment.

Importantly, such failures occur only in rare cases and do not reflect the general behavior of our system. Across most styles and identities, our approach maintains stable geometry, consistent textures, and coherent stylization across all novel views.

\section{Additional Results}
\cref{fig:additional-1,fig:additional-2} present the style reference images for a diverse set of artistic domains and the corresponding outputs produced by our model for multiple input identities.

\begin{figure*}[t!]
    \centering
    \includegraphics[width=1.0\linewidth]{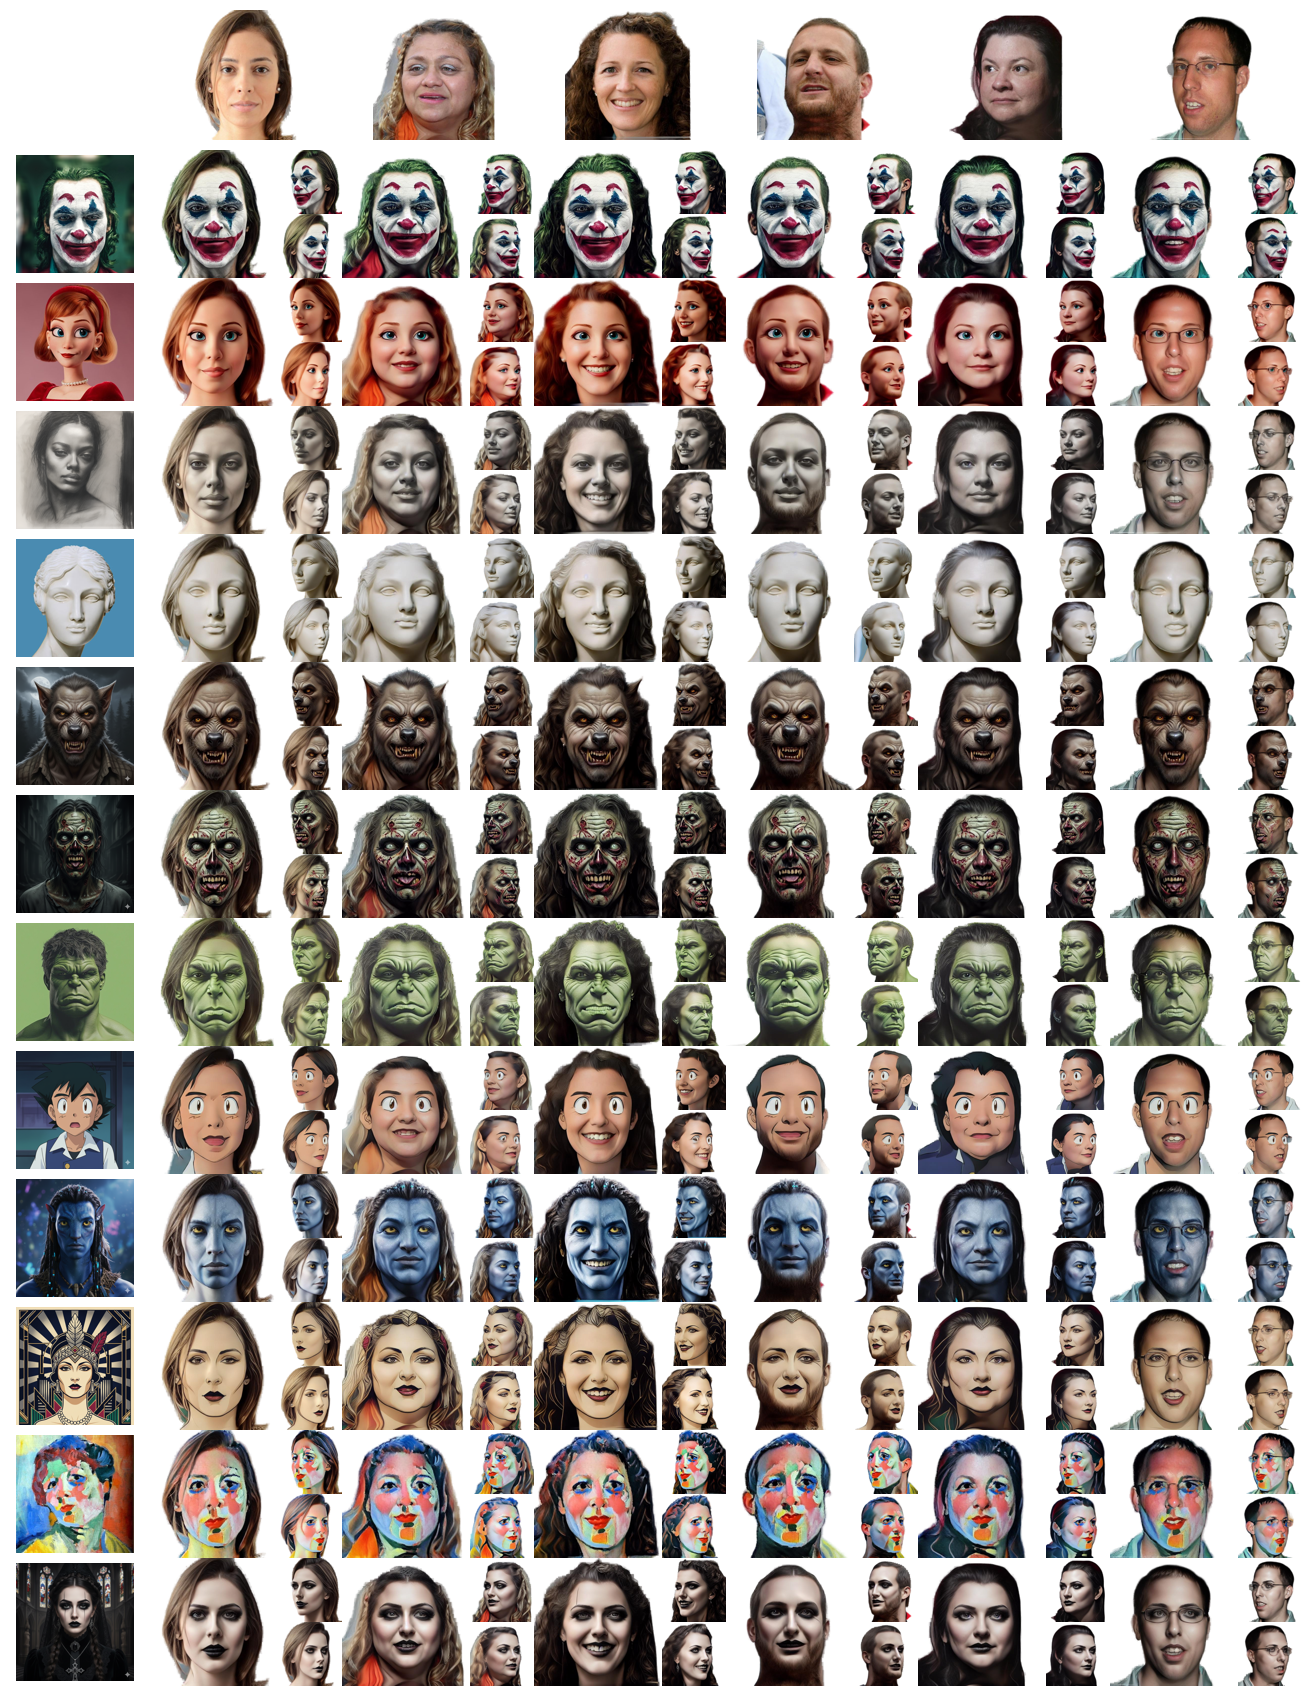}
      \vspace{-0.7cm}
    \caption{Additional qualitative results across a wide range of identities and style domains.}
    \label{fig:additional-1}
\end{figure*}

\begin{figure*}[t!]
    \centering
    \includegraphics[width=1.0\linewidth]{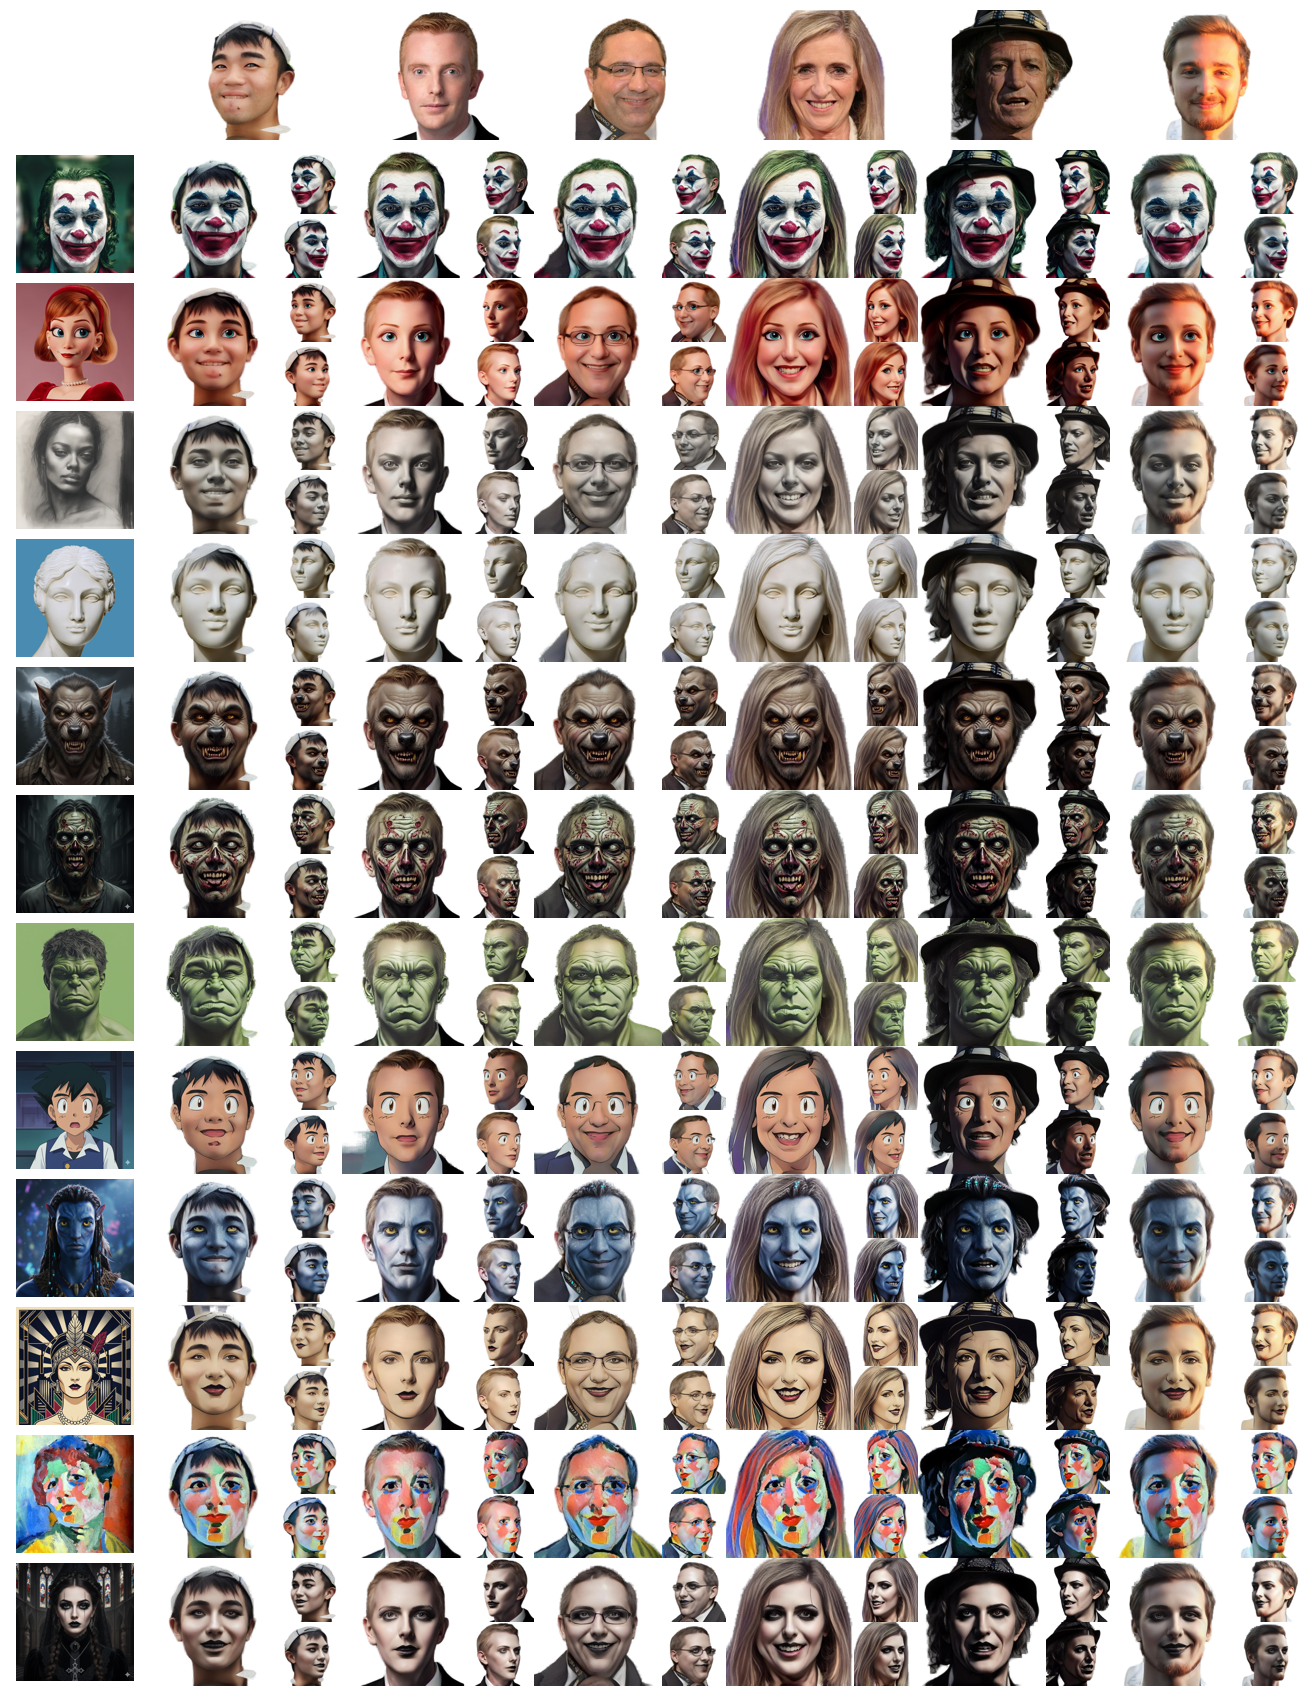}
      \vspace{-0.7cm}
    \caption{Additional qualitative results across a wide range of identities and style domains.}
    \label{fig:additional-2}
\end{figure*}
